# Supplementary material for: S-polarized light-sheets improve resolution and light-efficiency in oblique plane microscopy
Source: arXiv:2303.14018 source file (2023-12-14)
Supplement: Supplementary file 3 [file formating.tex]

\usepackage{authblk} % To use affiliations
\usepackage{graphicx} % Required for inserting images
\usepackage{lineno} % Line numbers
\usepackage{siunitx} % Required for alignment
\usepackage{upgreek} % Required for greek letters in text
\usepackage{cancel} % Required for crossing out text
\usepackage{varwidth} % Required for the text width of cells
\usepackage[utf8]{inputenc} % Required for special characters
\usepackage{amsmath,amsfonts,amssymb,amsthm,mathtools} % Required for some math elements
\usepackage[a4paper, total={7in, 9in}]{geometry}

%Packagaes for figures and tables
\usepackage{graphicx} % Graphics package
\usepackage{subcaption} % To have subfigures
\usepackage{wrapfig} % To wrap text around figures	
\usepackage{float} % To force figures to be placed in the right place

\usepackage{makeidx} % To make an index
\usepackage{color} % To use colors
\usepackage{hyperref} % To use hyperlinks
\usepackage{upgreek}

\usepackage[backend=biber,style=ieee,]{biblatex} % To use bibliography

\usepackage{siunitx}  %Write units easily \SI{value}

% To use code
\usepackage{listings} % To include code
\lstset{
basicstyle=\footnotesize\ttfamily,
identifierstyle=\bfseries\color{green!40!black},
commentstyle=\itshape\color{purple!40!black},
keywordstyle=\color{blue},
stringstyle=\color{orange}} % To set the style of the code

\usepackage{pdfpages} % To include pdf files
\usepackage{lscape} % To rotate pages

\usepackage{footnote} % To use footnotes
\usepackage{sidecap} % To use side captions
\usepackage{appendix} % To use appendices

% Table packages
\usepackage{tabularx} % To use tables
\makesavenoteenv{tabular} % To use footnotes in tables
\makesavenoteenv{table} % To use footnotes in tables
\usepackage{array} % To use tables
\usepackage{booktabs} % To use tables
 % To rotate text in tables

%Special in-document vector graphics:
\usepackage{tikz}
\usetikzlibrary{shapes.geometric,calc,positioning,3d,intersections,arrows}
\usetikzlibrary{decorations.markings}
\usepackage{pgfplots}
\pgfplotsset{compat=1.14}
\usepackage{circuitikz}  %Brukes til å enkelt tegne kretser

\usepackage{titling}
\setlength{\droptitle}{-8ex}
\pretitle{\begin{flushleft}\Large\bfseries}
\posttitle{\par\end{flushleft}}
\preauthor{\begin{flushleft}\Large}
\postauthor{\end{flushleft}}
\predate{\begin{flushleft}}
\postdate{\end{flushleft}}
% \usepackage{lineno}
% \linenumbers
